# Supplementary material for: Locality-Aware Hyperspectral Classification
Source: arXiv:2309.01561 source file (2023-09-04)
Supplement: Supplementary file 1 [file 6-supplementary.tex]

\section{Supplementary: Locality-Aware Hyperspectral Sensing}

%\mert{Once finished, we must generate two separate files, one for the main submission and one for the supplementary, not both in the same file!}

\partitle{Implementation Details.} The proposed Locality-Aware Hyperspectral Imaging Transformer is implemented with PyTorch. We adopt the backbone code from Hong et al.~\citep{hong2021spectralformer} and implement additional spatial attention modules and the regularization objective function. The experiments were run on NVIDIA RTX A6000 GPU. Our work strictly follows the experimental setup of Hong~\etal~\citep{hong2021spectralformer}, with identical train-test splits, hyper-parameters, datasets and metrics. The hyper-parameters are listed in Table \ref{tab:hyperpara}. We provide the details below. \textbf{CAF Layer}: To preserve the information across all layers, following~\citep{hong2021spectralformer}, we apply Cross-Adaptive Fusion (CAF) between the output of the previous $(l-2)$-th layer and the input of the current $(l)$-th layer. The representations of these two layers are fused with a $1 \times 2 $ convolution layer. We refer to Hong et al.~\citep{hong2021spectralformer} for more details. 

\partitle{Datasets.}  We evaluate our model on three standard, public benchmarks. \textit{i) \textbf{Indian Pines}~\citep{hyperdata}}: The dataset is collected by AVIRIS sensor over the Indian Pines test site in North-Western Indiana, USA. The dataset consists of $224$ spectral bands, sampled between $400-2500$ nm, with the spatial resolution of $145\times145$ pixels. The dataset includes $16$ distinct categories, $695$ training and $9671$ testing images. Typical categories include $\{corn, woods, wheat\}$. \textit{ii) \textbf{Houston2013}~\citep{houston2013}}: The dataset is collected by ITRES CASI-1500 sensor over the University of Houston campus. It contains $144$ spectral bands sampled between $380-1050$nm, with the spatial resolution of $349\times1905$ pixels. The dataset includes $15$ distinct categories, $2832$ training and $12197$ testing images. Typical categories include $\{water, soil, tree\}$. \textit{iii) \textbf{Pavia University}~\citep{hyperdata}}: The dataset is collected by ROSIS sensor over Pavia University, Italy. It contains $103$ spectral bands sampled between $430-860$nm, with the spatial resolution of $610\times340$ pixels. The dataset includes $9$ distinct categories, $3921$ training and $40002$ testing images. Typical categories include $\{asphalt, meadows, bricks\}$. 

\partitle{Baselines.} We compare our model to several state-of-the-art networks. The \textit{K-nearest neighbor} model makes predictions by calculating pairwise euclidean distance of spectral bands between training pixels~\citep{knn}. The \textit{random forest} classifier incorporates bagging of training pixels and random subspace feature selection of spectral bands~\citep{ham2005investigation}. The \textit{support vector machine} firstly projects spectral bands into high-dimensional feature space and maximises the geometrical margin between categories~\citep{melgani2004classification}. The \textit{1-D CNN} model performs 1-D convolution along spectral dimension~\citep{hu2015deep}, while the \textit{2-D CNN} model firstly patchifies the input image and then performs 2-D convolution along the spatial dimension~\citep{chen2016deep}. The \textit{RNN} model processes spectral bands as time sequences with a stack of recurrent layers and gated recurrent units~\citep{hang2019cascaded}. The \textit{miniGCN} network firstly generates adjacency matric with a KNN-based graph and then processed the generated graph via graph convolution layers~\citep{hong2020graph}. The \textit{ViT} based network uses ViT encoder blocks to process spectral bands as a sequence of signals~\citep{hong2021spectralformer}. Different from pure ViT, the \textit{SpectralFormer} patchifies the input image and groups neighboring spectral bands to a sequence of input vectors, and then processes the input via a stack of ViT encoder blocks~\citep{hong2021spectralformer}. Finally, \textit{MAEST} pretrains a feature exacter via a masked encoder-decoder reconstructing network and then fine-tunes the pretrained encoder with labeled data~\citep{ibanez2022masked}. Since the proposed LAHIT model is built upon SpectralFormer, we did not re-run all the baseline models except for the SpectralFormer and MAEST. Hence, we refer to Hong et al.~\citep{hong2021spectralformer} for more experimental details of those comparison baselines.

\partitle{Hyper-Parameter Tuning of $\lambda$.} According to the objective equation $($\ref{eq:loss}$)$ of the proposed \lahit{}, to find a suitable $\lambda$ that balances well between cross-entropy loss and local-spectral regularization loss, we evaluate \lahit{} with 6 different $\lambda$ values. The results are listed in Table \ref{tab:reg_weights}, which show that simply selecting $\lambda = 1$ works the best across most accuracy metrics.

\begin{table}[!ht]
\centering
\captionsetup{font=scriptsize}
\begin{minipage}{.5\linewidth}
\scalebox{0.65}{
\begin{tabular}{llll}
\hline
Class No. & Class Name      & Training & Testing \\ \hline
1         & Healthy Grass   & 198      & 1053    \\
2         & Stressed Grass  & 190      & 1064    \\
3         & Synthetic Grass & 192      & 505     \\
4         & Tree            & 188      & 1056    \\
5         & Soil            & 186      & 1056    \\
6         & Water           & 182      & 143     \\
7         & Residential     & 196      & 1072    \\
8         & Commercial      & 191      & 1053    \\
9         & Road            & 193      & 1059    \\
10        & Highway         & 191      & 1036    \\
11        & Railway         & 181      & 1054    \\
12        & Parking Lot1    & 192      & 1041    \\
13        & Parking Lot2    & 184      & 285     \\
14        & Tennis Court    & 181      & 247     \\
15        & Running Track   & 187      & 473     \\ \hline
          & Total           & 2832     & 12197   \\ \hline
\end{tabular}
}
\caption{Land-cover classes of Houston2013 dataset together with the training and testing samples for each class.}
\label{tab:Houston}
\end{minipage}%
\begin{minipage}{.5\linewidth}
\scalebox{0.65}{
\begin{tabular}{llll}
\hline
Class No. & Class Name   & Training & Testing \\ \hline
1         & Asphalt      & 548      & 6304    \\
2         & Meadows      & 540      & 18146   \\
3         & Gravel       & 392      & 1815    \\
4         & Trees        & 524      & 2912    \\
5         & Metal Sheets & 265      & 1113    \\
6         & Bare Soil    & 532      & 4572    \\
7         & Bitumen      & 375      & 981     \\
8         & Bricks       & 514      & 3364    \\
9         & Shadows      & 231      & 795     \\ \hline
          & Total        & 3921     & 40002   \\ \hline
\end{tabular}
}
\caption{Land-cover classes of Pavia University dataset together with the training and testing samples for each class.}
\label{tab:PU}
\end{minipage}
\end{table}

\begin{table}[!ht]
\centering
\captionsetup{font=scriptsize}
\scalebox{0.65}{
\begin{tabular}{llll}
\hline
Class No. & Class Name                   & Training & Testing \\ \hline
1         & Corn Notill                  & 50       & 1384    \\
2         & Corn Mintill                 & 50       & 784     \\
3         & Corn                         & 50       & 184     \\
4         & Grass Pasture                & 50       & 447     \\
5         & Grass Trees                  & 50       & 697     \\
6         & Hay Windrowed                & 50       & 439     \\
7         & Soybean Notill               & 50       & 918     \\
8         & Soybean Mintill              & 50       & 2418    \\
9         & Soybean Clean                & 50       & 564     \\
10        & Wheat                        & 50       & 162     \\
11        & Woods                        & 50       & 1244    \\
12        & Buildings Grass Trees Drives & 50       & 330     \\
13        & Stone Steel Towers           & 50       & 45      \\
14        & Alfalfa                      & 15       & 39      \\
15        & Grass Pasture Mowed          & 15       & 11      \\
16        & Oats                         & 15       & 5       \\ \hline
          & Total                        & 695      & 9671   \\ \hline
\end{tabular}
}
\caption{Land-cover classes of Indian Pines dataset together with the training and testing samples for each class.}
\label{tab:IP}
\end{table}

\begin{table}[!ht]
\centering
\captionsetup{font=scriptsize}
\begin{tabular}{ll}
\hline
Hyperparameter & Value                    \\ 
\midrule
Number of transformer blocks         & 5                   \\
Number of attention heads         & 4                    \\ 
Hidden dimension & 64 \\
Optimizer & Adam (weight decay=5e-3) \\
Initial learning rate  & 5e-4 \\
Learning rate scheduler & StepLR (gamma=0.9) \\
Batch size & 32 \\
Total training epoches & 300 \\ \hline
\end{tabular}
\caption{Hyperparameters of the architecture and training}
\label{tab:hyperpara}
\end{table}

\begin{table}[h]
\centering
\resizebox{\columnwidth}{!}{
\begin{tabular}{llllllllll}
\toprule

 & \multicolumn{3}{c}{Indian Pines} & \multicolumn{3}{c}{Houston2013} & \multicolumn{3}{c}{Pavia University} \\ 
 \cmidrule(lr){2-10} 

 $\lambda$ & OA & AA & Kappa & OA & AA & Kappa & OA & AA & Kappa \\ 
 \cmidrule(lr){2-4} \cmidrule(lr){5-7}  \cmidrule(lr){8-10}

0.1 & 86.96  & 91.68  & 0.85  & 84.27  & 86.06  & 0.83  & 83.25  & 89.63  & 0.79 \\ 
0.5 & 88.10 & 92.40 & 0.86 & 85.48 & 87.29 & 0.84 & 90.19 & 92.37 & 0.87 \\
\rowcolor{lightcyan} 1 & 89.80 & 94.69 & 0.88 & 88.49 & 89.74 & 0.86 & 91.28 & 92.25 & 0.88 \\ 
2 & 87.24 & 91.74 & 0.85 & 88.09 & 88.94 & 0.87 & 91.79 & 89.55 & 0.89 \\
5 & 87.01 & 93.28 & 0.85 & 85.18 & 86.67 & 0.84 & 81.70 & 90.65 & 0.77 \\
10 & 84.33 & 89.82 & 0.82 & 87.82 & 88.73 & 0.87 & 87.54 & 92.25 & 0.84 \\
\bottomrule
\end{tabular}}
\caption{Hyper-parameter tuning the magnitude of the regularization loss $(\lambda)$. Simply selecting $\lambda=1$ works best across most accuracy metrics.}
\label{tab:reg_weights}
\end{table}
